# Supplementary material for: Maxing Out the SVM: Performance Impact of Memory and Program Cache Sizes in the Agave Validator
Source: arXiv:2505.04129 source file (2025-05-07)
Supplement: Supplementary file 1 [file 9-appendix.tex]

\section{Appendix}

The Appendix contains an in-detail walkthrough of the execution and program cache implementation in the Agave Solana validator.

\subsection{Startup}
The core crate is the entry point for validator control flow in Solana. Its validator.rs file orchestrates startup logic, including the initialization of a TPU (Transaction Processing Unit). When the validator instance is instantiated, it creates a new TPU instance which initializes the core execution pipeline.
The TPU struct represents Solana’s transaction processing pipeline and consists of separate structs for each stage, including the BankingStage—where transaction execution occurs. This is where the BankingStage instance is instantiated and begins operation.
Transaction processing in the Banking Stage is driven by the BankingStage::process\_loop() function. This function loops continuously, calling the two key functions carrying out the responsibilities of the BankingStage:
\begin{enumerate}
    \item Fetching and buffering transactions: Handled by the receive\_and\_buffer\_packets() function, which collects incoming packets and organizes them for processing.
    \item Processing buffered transactions: Managed by process\_buffered\_packets(), which handles the actual execution of buffered packets.
\end{enumerate}

The BankingStage instance holds transactions in an UnprocessedTransaction instance. This structure separates transactions into two categories:
\begin{itemize}
    \item Vote transactions, stored in a VoteStorage instance.
    \item Non-vote transactions, stored in a ThreadLocalUnprocessedPackets instance.
\end{itemize}
Each thread in the \code{BankingStage} maintains its own \code{ThreadLocalUnprocessedPackets}, which wraps an \code{UnprocessedPacketBatches} instance. These batches, defined in unprocessed\_packet\_batches.rs, contain collections of PacketBatch objects, which represent the transactions arriving from the SigVerifyStage. For vote transactions, the data is handled separately by a vote \code{SigverifyStage} instance and stored in a corresponding \code{VoteStorage} instance.
By organizing transactions into these components, the BankingStage prepares data for efficient execution while maintaining flexibility for processing both vote and non-vote transactions.

\subsection{Execution Process Loop}

Execution in Solana involves a series of function calls that take transactions from the BankingStage, process them, and ultimately execute them within the Solana Virtual Machine (SVM). Below is an outline of the key steps in this flow:

\begin{enumerate}
  \item BankingStage (Handling Buffered Transactions)
  \begin{itemize}
    \item \code{BankingStage::process\_buffered\_packets()}: Determines whether to forward, hold, or consume incoming transactions based on the validator’s role and the bank’s state.
    \item \code{Consumer::consume\_buffered\_packets()}: Manages unprocessed transactions, iterating through vote and non-vote packets, and delegates packet processing to \code{do\_process\_packets()}.
  \end{itemize}

  \item Transaction Processing and Recording
  \begin{itemize}
    \item \code{Consumer::do\_process\_packets()}: Processes packets iteratively, enforcing slot timing constraints and collecting retryable transaction indices for reprocessing.
    \item \code{Consumer::process\_packets\_transactions()}: Filters expired retryable transactions and invokes \code{process\\_transactions()} while collecting relevant metrics.
    \item \code{Consumer::process\\_transactions()}: Processes transaction batches, identifies retryable failures, and enforces time and PoH constraints while recording trace-level results.
    \item \code{Consumer::process\_and\_record\_transactions()}: Performs transaction pre-execution checks for transaction validity.
    \item \code{Consumer::process\_and\_record\_transactions\_with\_pre\_results()}: Prepares and locks accounts, calculates transaction costs, handles retryable transactions, and forwards the batch for execution.
  \end{itemize}

  \item Executing and Committing Transactions
  \begin{itemize}
    \item \code{Consumer::execute\_and\_commit\_transactions\_locked()}: Executes and commits the transaction batch to the slot, ensuring a valid blockhash and recording to PoH.
    \item \code{Bank::load\_and\_execute\_transactions()}: Executes transactions via the SVM, identifying retryable transactions and logging execution details.
  \end{itemize}

  \item SVM Execution
  \begin{itemize}
    \item \code{TransactionBatchProcessor::load\_and\_execute\_sanitized\_transactions()}: Loads programs, executes transactions, and manages the program cache.
    \item \code{TransactionBatchProcessor::execute\_loaded\_transaction()}: Prepares transaction state, executes via the SVM, and collects execution results.
    \item \code{MessageProcessor::process\_message()}: Prepares transaction state, executes via the SVM, and collects execution results.
  \end{itemize}

  \item Instruction Execution in the Virtual Machine
  \begin{itemize}
    \item \code{InvokeContext::process\_instruction()}: Passes control to \code{process\_executable\_chain()} to begin execution within the SVM.
    \item \code{InvokeContext::process\_executable\_chain()}: Instantiates an eBPF VM, finds the program entrypoint, and executes the program.
    \item \code{solana\_rbpf::vm::invoke\_function()}: Instantiates an eBPF VM, finds the program entrypoint, and executes the program.
  \end{itemize}
\end{enumerate}

An in-depth walkthrough of every function call is in the appendix.

\subsection{Execution Call-by-Call}

Execution occurs in a series of fifteen function calls ranging from the banking stage to the SVM and ending in the eBPF virtual machine. The following gives a detailed description of every call and its functionality, along with the structures that orchestrate the process.

core::banking\_stage.rs::BankingStage::process\_buffered\_packets()

This is the first significant step in the transaction execution flow. It determines the appropriate action for packets in the buffer based on the validator’s current role and status:
\begin{itemize}
    \item \code{Forward}: If the validator is neither the leader nor about to become one, the packet is forwarded to the current leader.
    \item \code{ForwardAndHold}: If the validator is not yet the leader but will assume the role shortly, packets are both forwarded to the leader and retained in the local buffer for potential processing.
    \item \code{Hold}: If the validator is the leader and the bank has not yet been initialized, packets are held in the buffer.
    \item \code{Consume}: If the validator is the current leader and the bank is active, the packets are consumed by invoking Consumer::consume\_buffered\_packets().
\end{itemize}

This decision-making process uses the \code{DecisionMaker} instance to analyze the validator’s status and take the corresponding action. By effectively segregating packets into these categories, Solana ensures efficient handling of transactions under varying validator roles.

\code{core::banking\_stage::consumer.rs::Consumer::consume\_buffered\_packets()}

Once the decision is made to process packets, execution flow is handed off to the Consumer instance in the banking\_stage module in the core crate. This method is responsible for processing all packets in the buffer.

\begin{itemize}
    \item -	It calls process\_packets() on the UnprocessedTransactionStorage instance, which holds the packets to be processed.
    \item A processing function, Consumer::do\_process\_packets(), is passed to process\_packets() as a callback.
    \item process\_packets() distinguishes between two types of storage:
    \begin{itemize}
        \item VoteStorage: Processes vote transactions.
        \item LocalTransactionStorage: Handles non-vote transactions.
    \end{itemize}
\end{itemize}

This separation ensures that vote and non-vote transactions are handled appropriately.

\code{core::banking\_stage::consumer.rs::Consumer::do\_process\_packets()}

\code{do\_process\_packets()} is where packet processing begins. It performs several checks and actions for each packet in the buffer:

\begin{enumerate}
  \item End of Slot Check: If the current slot has ended, the function immediately returns, halting further processing.
  \item Process Transactions: For each packet, it invokes \code{process\_packet\_transactions()}, which processes the transactions within that packet.
  \item Slot Processing Limits:
  \begin{itemize}
    \item It checks whether the maximum PoH height has been reached or if the allocated transaction ingestion time (set by the \code{ns\_per\_slot} field in the Bank) has expired.
    \item These checks use the method \code{poh::poh\_recorder.rs::BankStart::should\_working\_bank\_still\_be\_processing\_txs()} to compare the current state with the Bank’s \code{should\_still\_be\_processing\_txns()} logic.
  \end{itemize}
  \item Retryable Indices: If a transaction cannot currently be processed (e.g., due to insufficient resources or missing dependencies), its index is added to a vector of retryable indices, allowing for future reprocessing.
\end{enumerate}

This function enforces timing constraints and ensures that packets are processed efficiently while respecting the slot’s boundaries. Once processing is complete, execution is handed off to \code{process\_packets\_transactions()} for transaction-level handling.

\code{core::banking_stage::consumer.rs::Consumer::process_packets_transactions()}
\code{process_packets_transactions()} calls \code{process_transactions()} to handle transaction execution and then filters expired retryable transactions while collecting relevant metrics. The function’s return type provides insight into the stage of execution being handled:

\begin{enumerate}
  \item Retryable transactions: Transactions that failed due to temporary errors like \code{AccountInUse} lock conflicts or \code{CostModel} compute limits. These are added to \code{retryable\_transaction\_indexes} for reprocessing.
  \item Dropped transactions: Transactions that failed due to fatal errors such as being too old or having duplicate signatures. These are removed from the processing queue and are not retryable.
  \item Committed transactions: Transactions successfully executed and committed to the Bank. These are counted in \code{committed\_transactions\_count}.
  \item Failed commit transactions: Transactions that executed but failed to commit. These are counted in \code{failed\_commit\_count}.
\end{enumerate}

\code{core::banking_stage::consumer.rs::Consumer::process_transactions()}

\code{process_transactions()} collects the results of processing transaction batches and identifies transactions that failed but are eligible for retries, adding them to a retryable transaction vector. For each batch of transactions, it calls \code{process_and_record_transactions()}. This function enforces time and PoH constraints by breaking out early if the Bank’s transaction processing window or PoH height limit is reached. 

\code{core::banking\_stage::consumer.rs::Consumer::process\_and\_record\_transactions()}

In \code{process_and_record_transactions()}, transactions undergo pre-execution checks to ensure they haven’t already been processed. These checks involve calling \code{bank.check\_transactions()} (to verify age and if the transaction has already been processed) and then verifying precompiles. If the transactions pass these verifications, execution is handed off to \code{process_and_record_transactions_with_pre_results()}.

\code{core::banking\_stage::consumer.rs::Consumer::process\_and\_record\_transactions\_with\_pre\_results()}

\code{process\_and\_record\_transactions\_with\_pre\_results()} prepares transactions for execution by locking accounts and determining their costs. Here is a step-by-step breakdown:

\begin{enumerate}
  \item Transaction Cost Selection: Calls \code{QosService::select\_and\_accumulate\_transaction\_costs()} to evaluate the transaction costs of the sanitized transactions passed in.
  \item Account Locking: Calls \code{bank.prepare\_sanitized\_batch\_with\_results()}, which locks the necessary accounts and identifies whether transactions can proceed or need to be retried. Transactions encountering specific limits (e.g., \code{AccountInUse} or \code{WouldExceedMaxBlockCostLimit}) are marked as retryable.
  \item Batch Execution: The prepared transaction batch is passed to \code{execute\_and\_commit\_transactions\_locked()} for execution and commitment to the Bank.
  \item Cost Adjustment: After execution, \code{QosService::remove\_or\_update\_costs()} adjusts transaction costs based on actual outcomes, such as aborted or unexecuted transactions.
\end{enumerate}

\code{core::banking\_stage::consumer.rs::Consumer::execute\_and\_commit\_transactions\_locked()}

This function is responsible for executing the transaction batch and committing the results. Key steps include:

\begin{enumerate}
  \item Collect Metadata: Gathers token and account balances and determines compute budgets for the transactions.
  \item Transaction Execution: Calls \code{bank.load\_and\_execute\_transactions()} to execute the transactions.
  \item Blockhash Race Condition Avoidance: Fetches the last valid blockhash via \code{bank.last\_blockhash\_and\_lamports\_per\_signature()} to prevent race conditions where the blockhash queue advances during transaction commitment, leading to invalid blockhash mismatches.
  \item Transaction Recording: Sends transactions to be recorded in the slot’s Proof of History (PoH) via \code{transaction\_recorder.record\_transactions()}.
  \item Commit Transactions: Invokes \code{committer.commit\_transactions()} to finalize the transactions into the block.
  \item Metrics and Logging: Records performance metrics, logs processing times, and emits debug-level outputs for execution details.
\end{enumerate}

This function processes transaction batches, ensuring that transactions are either executed or aborted and appropriately classified as retryable.

\begin{enumerate}
  \item Transaction Lock Results: Determines lock conflicts and marks the following transactions as retryable:
  \begin{itemize}
    \item \code{AccountInUse}
    \item \code{WouldExceedMaxBlockCostLimit}
    \item \code{WouldExceedMaxVoteCostLimit}
    \item \code{WouldExceedMaxAccountCostLimit}
    \item \code{WouldExceedAccountDataBlockLimit}
  \end{itemize}

  \item Validation: Calls \code{check\_transactions()}, which includes:
  \begin{itemize}
    \item \code{check\_age()} – Ensures transactions are within the valid execution window.
    \item \code{check\_status\_cache()} – Calls \code{is\_transaction\_already\_processed()} to prevent duplicate execution.
  \end{itemize}

  \item Execution via SVM: Calls \code{load\_and\_execute\_sanitized\_transactions()} on each transaction in the batch, which is the Bank’s entry point into the Solana Virtual Machine (SVM).

  \item Logging: Collects transaction execution logs, including:
  \begin{itemize}
    \item Accounts used
    \item Transaction signatures
    \item Error summaries
    \item Debug-level logs detailing failures and retries.
  \end{itemize}
\end{enumerate}

\code{svm::transaction\_processor.rs::TransactionBatchProcessor::load\_and\_execute\_sanitized\_transactions()}
This function orchestrates transaction execution by interacting with the program cache, loading accounts, and executing transactions.

\begin{enumerate}
  \item Validate Transaction Fees: Calls \code{validate\_fees()} on all transactions in the batch.

  \item Prepare Program Cache:
  \begin{itemize}
    \item Fetches executable program accounts and built-in programs needed for the batch.
    \item Calls \code{replenish\_program\_cache()} to initialize \code{ProgramCacheForTxBatch}, ensuring the program cache is populated for execution.
  \end{itemize}

  \item Load Accounts: Retrieves the necessary accounts from the program cache.

  \item Transaction Execution: Iterates through the transactions and calls \code{execute\_loaded\_transaction()} for each.

  \item Cache Management:
  \begin{itemize}
    \item If the batch increases the program cache size, \code{evict\_using\_2s\_random\_selection()} is called to evict programs using the 2’s random selection strategy, reducing cache size to 90\% of capacity.
  \end{itemize}
\end{enumerate}

\code{svm::transaction\_processor.rs::TransactionBatchProcessor::execute\_loaded\_transaction()}
This function handles the execution of an individual transaction, preparing account states and invoking execution.

\begin{enumerate}
  \item Compute Budget \& Context Setup:
  \begin{itemize}
    \item Computes rent, lamports, and compute budget requirements.
    \item Initializes a \code{TransactionContext} to manage execution state (instruction stack depth, trace length, etc.).
  \end{itemize}

  \item Pre-Execution State Collection: Captures initial rent, lamports in accounts, and other state data.

  \item Invoke Context Creation: Instantiates an \code{InvokeContext} to track execution context and handle cross-program invocations.

  \item Transaction Execution: Calls \code{MessageProcessor::process\_message()} to execute the transaction.

  \item Post-Execution State Collection: Gathers results, including execution status, logs, and final account states.
\end{enumerate}

\code{svm::message\_processor.rs::MessageProcessor::process\_message()}
This function processes each instruction within a transaction, ensuring Bank constraints are met and invoking execution logic.

\begin{enumerate}
  \item Instruction Iteration: Iterates through all instructions in the transaction’s \code{SanitizedMessage}, ensuring validity.
  \item Banking Rule Enforcement: Checks each instruction against Bank accounting rules.
  \item Instruction Metadata Tracking: Assigns an \code{InstructionAccount} instance to each instruction to manage execution metadata.
  \item Instruction Execution: Calls \code{InvokeContext::process\_instruction()} to execute each instruction in the message.
\end{enumerate}

program-runtime::invoke\_context.rs::InvokeContext::process\_instruction()

This function serves as the entry point into the program\_runtime crate for executing a single instruction.

\begin{enumerate}
  \item Delegates Execution: Calls \code{process\_executable\_chain()} to begin execution within the Solana Virtual Machine (SVM).
  \item Manages Execution Context: Ensures that execution occurs within the correct program execution environment.
  \item Handles Cross-Program Calls: If the instruction invokes another program, ensures proper setup and execution.
\end{enumerate}

\code{program-runtime::invoke\_context.rs::InvokeContext::process\_executable\_chain()}

This function calls the on-chain program’s entrypoint method.

\begin{enumerate}
  \item Program Entry Point Resolution:
  \begin{itemize}
    \item Searches for the program’s entrypoint function by checking for the hashed value \code{"entrypoint"}.
    \item Ensures the program binary is loaded and ready for execution.
  \end{itemize}

  \item eBPF Virtual Machine Setup:
  \begin{itemize}
    \item Instantiates a new eBPF virtual machine (vm) using:
    \item \code{ProgramBatchForTransaction} (batch of loaded programs),
    \item \code{ProgramRuntimeEnvironment} (execution environment),
    \item \code{InvokeContext} (execution state and metadata).
  \end{itemize}

  \item Execution Invocation:
  \begin{itemize}
    \item Calls \code{vm.invoke\_function()} to execute the program within the eBPF VM.
  \end{itemize}

  \item Retrieve Execution Results:
  \begin{itemize}
    \item Captures return values via memory-mapped structures in the VM.
    \item Accounts for compute units consumed.
  \end{itemize}

  \item Error Handling \& Metrics:
  \begin{itemize}
    \item Collects execution metrics (compute units, instruction counts).
    \item Logs execution errors and failure states.
  \end{itemize}
\end{enumerate}

solana\_rbpf::vm::invoke\_function()

This function is the core execution mechanism within Solana’s eBPF virtual machine.

\begin{enumerate}
  \item Execute the Program:
  \begin{itemize}
    \item Calls the function defined in the transaction.
    \item Runs in an isolated eBPF environment with restricted system calls.
  \end{itemize}

  \item Store Execution Result:
  \begin{itemize}
    \item The result of the function execution is stored in \code{vm.program\_result}.
  \end{itemize}

  \item Enforces Compute Budget:
  \begin{itemize}
    \item Execution is halted if the compute budget (CU limit) is exceeded.
  \end{itemize}
\end{enumerate}

\subsection{Program Cache Implementation}

The program cache is implemented as a hierarchy of structs that efficiently manage and track loaded programs. Below, we describe the key components of the ProgramCache struct, its related members, and how it organizes and tracks data.

ProgramCache struct
The ProgramCache struct is the top-level structure encapsulating the program cache. It manages the lifecycle of all loaded programs and coordinates interactions with other components of the validator, such as the Bank and the SVM. The cache is generic over a type that implements the ForkGraph trait, allowing it to reference the broader state of the chain, including forks and re-rootings.
Key Members of ProgramCache
index (IndexImplementation)
The primary index for the cache. It maps program IDs to their corresponding ProgramCacheEntry. The index also tracks usage statistics for each program, such as access frequency and load counts.
latest\_root\_slot (Slot)
Tracks the most recent slot for which the program cache was rooted. This ensures that the cache operates in sync with the validator’s fork structure.
latest\_root\_epoch (Epoch)
Stores the most recent epoch for which the cache was rooted. 
runtime\_environments
Manages the invocation context for programs being executed in the current epoch. Each runtime environment contains the necessary metadata and state for executing eBPF bytecode.
upcoming\_environments
Used only at epoch boundaries to warm the program cache in anticipation of the next epoch. This mechanism allows the new epoch to inherit a warm execution environment, reducing latency when the epoch transitions.
programs\_to\_recompile
A list of programs that need to be recompiled before the next epoch. This ensures that the cache stays consistent with updates to program bytecode.
stats (ProgramCacheStats)
Tracks cache performance metrics, such as:

\begin{itemize}
    \item Number of program loads
    \item Cache hits and misses
    \item Evictions (via 2’s random eviction)
\end{itemize}

These statistics are critical for diagnosing performance bottlenecks and tuning the cache’s behavior.

fork\_graph (FG: ForkGraph)
A reference to the block store. This is used to handle forks and ensure the program cache correctly reflects the state of the chain.

loading\_task\_waiter
Coordinates transaction batches that are awaiting a program load due to contention. This enables cooperative loading during parallel execution, avoiding redundant work when multiple threads need the same program.

IndexImplementation: Organizing and Tracking Cached Programs
The next level down into the cache is the index, an instance of IndexImplementation, which holds two HashMaps: entries and loading\_entries. loading\_entries keeps track of programs that are being loaded; entries organize programs that are loaded. The Hashmap relates public keys to a program: each public key is mapped to a Vec which holds the version of a program at a slot.

The IndexImplementation is the backbone for organizing and tracking all loaded and currently-loading programs in the cache. It uses HashMaps to efficiently map public keys (program identifiers) to their corresponding versions and metadata.

The IndexImplementation struct manages two primary HashMaps for efficient lookup and coordination during program loading and execution:
entries (HashMap<Pubkey, Vec>)

Tracks programs that are already loaded into the cache.

\begin{itemize}
    \item Each public key (Pubkey) corresponds to a vector (Vec) containing all the program versions at different slots. This ensures that the cache can handle forks and state changes efficiently.
    \item Example: A public key might map to multiple versions of a program, reflecting its state across different forks.
\end{itemize}

loading\_entries (HashMap<Pubkey, Vec>)
Tracks programs currently being loaded into the cache.

\begin{itemize}
    \item While a program is being loaded (e.g., from disk to memory), it is temporarily tracked in loading\_entries. This prevents duplicate work when multiple threads or transactions require the same program. The loading\_entries HashMap ensures that:
    \begin{itemize}
        \item Only one thread loads a program at any given time.
        \item -	Other threads waiting for the program are notified once the loading is complete.
    \end{itemize}
    \item Each LoadingState entry is:
    \begin{itemize}
        \item Key: the public key of the program.
        \item Value: A tuple of the slot of the program being loaded and the thread that is doing the loading.
    \end{itemize}
\end{itemize}

ProgramCacheEntry and ProgramCacheEntryType
Each program in the cache is represented by the ProgramCacheEntry struct, which encapsulates a specific version of a program for a specific slot with associated metadata. This struct is critical for managing program state, ensuring accurate execution, and optimizing cache performance.
Because the ProgramCacheEntry is specific to a slot and, by extension, a fork, the program cache maintains correct execution even in the presence of fork-specific differences. In other words, the correct version of a program is executed for any given slot and fork.

State Representation via ProgramCacheEntryType
A ProgramCacheEntry represents the state of a program using the ProgramCacheEntryType enum, which defines various possible states of a program in the cache. These states include:

\begin{figure}[tbp]
    \centering
    \footnotesize
\begin{tabular}{|l|p{9cm}|}
\hline
\textbf{State} & \textbf{Description} \\
\hline
\code{FailedVerification} & The program failed validation and cannot currently be executed. It remains in the cache as a tombstone in case a future feature set change makes it valid. \\
\hline
\code{Closed} & Also used for program loader accounts (e.g., buffer accounts for LoaderV3) that don’t contain executable code. \\
\hline
\code{DelayVisibility} & Represents programs that have been modified but whose updated versions are not yet visible. \\
\hline
\code{Unloaded} & Programs that are no longer compiled but still track usage statistics (e.g., for eviction purposes). \\
\hline
\code{Loaded} & The primary state for programs actively used in transactions. These programs are verified, compiled, and ready for execution. \\
\hline
\code{Builtin} & Programs built into the validator itself, such as the system program, which are not stored on-chain but are distributed with the validator. \\
\hline
\end{tabular}
    \caption{Caption}
    \label{fig:enter-label}
\end{figure}

Program-Specific Metadata

Alongside the program itself, the ProgramCacheEntry holds metadata essential for managing and tracking program execution, including:

\begin{figure}[tbp]
    \centering
    \footnotesize
\begin{tabular}{|l|p{6cm}|}
\hline
\textbf{Field} & \textbf{Description} \\
\hline
\code{program}: \code{ProgramCacheEntryType} & Represents the current state of the program within the cache, as defined by the \code{ProgramCacheEntryType} enum (Loaded, Unloaded, FailedVerification, Closed, etc). Tracks the operational status of the program and ensures the validator knows how to handle it during execution. \\
\hline
\code{account_owner}: \code{ProgramCacheEntryOwner} & The public key of the account that owns the program. Ensures the validator can verify ownership of the program and enforce proper execution rules. \\
\hline
\code{account_size}: \code{usize} & The size of the account that stores the program and its associated data, in bytes. Allows the validator to track memory usage and make informed eviction decisions when managing cache capacity. \\
\hline
\code{deployment_slot}: \code{Slot} & The slot in which the program was deployed or last redeployed. Provides historical context for the program’s lifecycle, helping manage fork-specific state. \\
\hline
\code{effective_slot}: \code{Slot} & The slot in which the program becomes active and can be executed. This slot may be in the future relative to the current block height. Ensures that programs are only executed when they are valid and active according to their deployment rules. \\
\hline
\code{tx_usage_counter}: \code{AtomicU64} & Tracks how often this program entry has been used in transactions. Uses an atomic counter for thread-safe updates in a multithreaded environment. Provides usage statistics that inform eviction policies (e.g., least frequently used). \\
\hline
\code{ix_usage_counter}: \code{AtomicU64} & Tracks how often this program entry has been used in instructions. Like \code{tx\_usage\_counter}, it uses an atomic counter for safe concurrent updates. Differentiates between usage in transactions and direct instruction invocations for granular tracking. \\
\hline
\code{latest_access_slot}: \code{AtomicU64} & Records the most recent slot in which the program entry was accessed. Helps the cache track recency of access, enabling eviction strategies like least recently used (LRU) or other hybrid policies. \\
\hline
\end{tabular}
    \caption{Caption}
    \label{fig:enter-label}
\end{figure}

This allows the following to be managed by the cache:

\begin{itemize}
  \item Program state via \code{program}.
  \item Ownership and resource usage via \code{account\_owner} and \code{account\_size}.
  \item Lifecycle and activity via \code{deployment\_slot}, \code{effective\_slot}, and \code{latest\_access\_slot}.
  \item Usage patterns via \code{tx\_usage\_counter} and \code{ix\_usage\_counter}.
\end{itemize}

Executable, Builtin and ELF programs in the Program Cache

In the ProgramCacheEntryType enum, the Loaded and Builtin variants represent active, executable programs within the Solana validator. These programs exist in two distinct forms: ELF-based executables and builtin programs. 

When a program is loaded into the cache, it must be in one of two formats:

\begin{itemize}
  \item ELF Executables (\code{Executable}): JIT-compiled or interpreted eBPF bytecode.
  \item Builtin Programs (\code{BuiltinProgram}): Hardcoded system programs that do not exist on-chain.
\end{itemize}

ELF Executables (Executable)

Defined in elf.rs (within the solana\_rbpf crate), ELF executables represent dynamically loaded programs compiled into machine code. These are smart contracts deployed by users and executed by the validator.

ELF executables are:

\begin{itemize}
  \item Loaded from on-chain account storage when a transaction invokes the program.
  \item Either JIT-compiled to the validator’s native machine code or interpreted via the eBPF virtual machine.
  \item Cached in \code{ProgramCacheEntry} so that it does not need to be reloaded for subsequent transactions.
  \item Associated with \code{InvokeContext}, which manages execution state.
\end{itemize}

Loading and execution of ELF executables:

\begin{itemize}
  \item Programs are compiled and executed in the \code{solana\_rbpf} virtual machine.
  \item The ELF program defines an entrypoint, which the validator searches for using \code{process\_executable\_chain()} in \code{invoke\_context.rs}.
  \item Programs are subject to compute budgets, which determine resource allocation.
\end{itemize}

\point{Builtin Programs (BuiltinProgram)}
Defined in program.rs (within the solana\_rbpf crate), builtin programs are preloaded into the validator’s execution environment and are not stored on-chain.
Builtin programs are:

\begin{itemize}
  \item Hardcoded into the validator binary and distributed with each Solana release.
  \item Used for core validator logic, such as:
  \begin{itemize}
    \item System Program (creating accounts, transferring SOL)
    \item Stake Program (handling stake accounts)
    \item Vote Program (processing validator votes)
  \end{itemize}
  \item Unlike ELF executables, builtin programs do not need to be loaded from account storage.
\end{itemize}

Execution flow for builtin programs

\begin{itemize}
  \item When a transaction invokes a builtin program, the validator instantly resolves it without fetching data from disk.
  \item Execution happens directly within the validator.
  \item Like ELF executables, \code{InvokeContext} is used to track execution state.
\end{itemize}

Runtime Implementation

ProgramRuntimeEnvironment

Each cached program is associated with a ProgramRuntimeEnvironment instance. This structure encapsulates execution metadata and ensures a consistent environment for transactions; it defines the runtime state in which programs execute.

A ProgramRuntimeEnvironment does:

\begin{itemize}
  \item Maintains compiled versions of the program (JIT-compiled or interpreted).
  \item Tracks execution metadata, including:
  \begin{itemize}
    \item Compute budgets (limits on execution resources).
    \item Program dependencies (e.g., system calls, imported libraries).
    \item Execution state across forks.
  \end{itemize}
\end{itemize}

This structure ensures the correct execution environment for both ELF and builtin programs and reduces redundant program recompilations.

InvokeContext

Defined in invoke\_context.rs (within the program\_runtime crate), InvokeContext is responsible for tracking the state of a transaction as it executes within the Solana Virtual Machine (SVM). It manages:

\begin{itemize}
  \item Instruction Execution – Tracks the instruction currently being executed.
  \item Compute Budgeting – Ensures transactions adhere to compute limits.
  \item Cross-Program Invocations – Supports program-to-program calls.
  \item Account Access – Controls read/write access to accounts.
  \item Error Handling – Captures execution failures and propagates errors.
  \item Syscall Contexts – Stores execution contexts for system calls.
\end{itemize}

Mapped to the fields of the struct, this looks like:

Transaction \& Program Context

\begin{itemize}
  \item \code{transaction\_context}: \code{\&'a mut TransactionContext}: Tracks information about the currently executing transaction. This includes accounts, instructions, and program execution state.
  \item \code{program\_cache\_for\_tx\_batch}: \code{\&'a mut ProgramCacheForTxBatch}: Caches loaded programs for the entire transaction batch. Prevents redundant loads within the same batch.
\end{itemize}

Compute Budget \& Execution Limits

\begin{itemize}
  \item \code{compute\_budget}: \code{ComputeBudget}: Defines the maximum compute units a transaction is allowed to consume.
  \item \code{compute\_meter}: \code{RefCell<u64>}: Tracks compute units already consumed during execution. If \code{compute\_meter} exceeds \code{compute\_budget}, execution fails.
\end{itemize}

Logging \& Execution Profiling

\begin{itemize}
  \item \code{log\_collector}: \code{Option<Rc<RefCell<LogCollector>>>}: Collects logs generated by the program during execution. Used for debugging and transaction tracing.
  \item \code{execute\_time}: \code{Option<Measure>}: Measures the time spent executing the program.
  \item \code{timings}: \code{ExecuteDetailsTimings}: Stores fine-grained execution timing details, used for performance monitoring.
\end{itemize}

Syscall Handling

\begin{itemize}
  \item \code{syscall\_context}: \code{Vec<Option<SyscallContext>>}: Holds syscall state for execution. Programs interact with the runtime through syscalls, such as logging, account access, or cross-program invocation.
\end{itemize}

Tracing \& Debugging

\begin{itemize}
  \item \code{traces}: \code{Vec<Vec<[u64; 12]>>}: Stores execution traces, capturing key performance and execution events. These traces provide low-level insights into how a program executes on the validator.
\end{itemize}

Interaction Between InvokeContext and ProgramRuntimeEnvironment in the Execution Pipeline

\begin{enumerate}
  \item Fetch the Cached Program (\code{TransactionBatchProcessor::load\_and\_execute\_sanitized\_transactions()})
  \begin{enumerate}
    \item Execution begins in \code{TransactionBatchProcessor::load\_and\_execute\_sanitized\_transactions()}, which:
    \begin{itemize}
      \item Looks up the program in the Program Cache (\code{ProgramCacheForTxBatch}).
      \item If found, retrieves the \code{ProgramRuntimeEnvironment} containing the compiled program.
      \item If the program is missing, it must be loaded into the cache.
    \end{itemize}
  \end{enumerate}

  \item Provision the Execution Context (\code{TransactionBatchProcessor::execute\_loaded\_transaction()})
  \begin{enumerate}
    \item A new \code{InvokeContext} is instantiated for the transaction.
    \item This happens in \code{TransactionBatchProcessor::execute\_loaded\_transaction()}.
    \item It initializes:
    \begin{itemize}
      \item The transaction state (\code{TransactionContext}).
      \item A reference to the program cache (\code{ProgramCacheForTxBatch}).
      \item Execution constraints: \code{ComputeBudget}, \code{SyscallContext}, and logging.
      \item This ensures the execution adheres to compute budgets and fork-aware execution rules.
    \end{itemize}
  \end{enumerate}

  \item Execute Instructions (\code{MessageProcessor::process\_message()} $\rightarrow$ \code{InvokeContext::process\_instruction()})
  \begin{enumerate}
    \item The execution of instructions begins in \code{MessageProcessor::process\_message()}.
    \item Each instruction within the transaction is processed in sequence.
    \item \code{InvokeContext::process\_instruction()} is called for each instruction.
    \item If the program being executed is an on-chain eBPF program, execution is delegated to the eBPF virtual machine.
  \end{enumerate}

  \item Invoke the Program \& Execute eBPF Code (\code{InvokeContext::process\_executable\_chain()} $\rightarrow$ \code{solana\_rbpf::vm::invoke\_function()})
  \begin{enumerate}
    \item \code{InvokeContext::process\_executable\_chain()} is called.
    \item It finds the program entrypoint by searching for the hashed “entrypoint” symbol.
    \item A new eBPF virtual machine (VM) is instantiated.
    \item The function \code{solana\_rbpf::vm::invoke\_function()} is called, executing the program’s bytecode.
    \item The \code{ProgramRuntimeEnvironment} provides JIT-compiled or interpreted program execution.
  \end{enumerate}

  \item Track Compute \& Enforce Limits (\code{InvokeContext::compute\_meter})
  \begin{enumerate}
    \item The \code{compute\_meter} inside \code{InvokeContext} tracks execution cost:
    \begin{itemize}
      \item Every instruction execution updates compute units consumed.
      \item If a program exceeds its compute budget, execution terminates immediately.
    \end{itemize}
  \end{enumerate}

  \item Finalizing Execution \& Logging (\code{TransactionBatchProcessor::execute\_loaded\_transaction()})
  \begin{enumerate}
    \item The program execution returns to \code{InvokeContext::process\_instruction()}.
    \item Post-execution state tracking occurs:
    \begin{itemize}
      \item Updates the program’s usage counters in \code{ProgramCacheEntry}.
      \item Logs transaction execution results.
      \item Stores execution traces in \code{InvokeContext::traces}.
    \end{itemize}
  \end{enumerate}

  \item Return Execution Results to Bank (\code{Bank::load\_and\_execute\_transactions()})
  \begin{enumerate}
    \item After all transactions in the batch are processed:
    \begin{itemize}
      \item The \code{InvokeContext} finalizes compute costs.
      \item Transaction results are returned to the Bank, which updates the validator’s state.
    \end{itemize}
  \end{enumerate}
\end{enumerate}

Loading of Executables into the Cache

When a new program is loaded into the Program Cache, it is wrapped in a ProgramCacheEntry. Every ProgramCacheEntry (except tombstones) holds an executable that will be used during execution.

Instantiating a New ProgramCacheEntry

When a new ProgramCacheEntry is created, the constructor ProgramCacheEntry::new() is called. This leads to a call to new\_internal(), which initializes the entry with the following parameters:

\begin{tabular}{|l|p{10cm}|}
\hline
\textbf{Field} & \textbf{Description} \\
\hline
\code{loader\_key}: \code{\&Pubkey} & The public key of the program loader. \\
\hline
\code{program\_runtime\_environment}: \code{Arc<BuiltinProgram<InvokeContext<'static>>>} & The runtime environment containing metadata for execution. \\
\hline
\code{deployment\_slot}: \code{Slot} & The slot where the program was deployed. \\
\hline
\code{effective\_slot}: \code{Slot} & The slot at which the program becomes active. \\
\hline
\code{elf\_bytes}: \code{\&[u8]} & The raw ELF bytecode of the program. \\
\hline
\code{account\_size}: \code{usize} & The size of the account storing the program data. \\
\hline
\code{metrics}: \code{\&mut LoadProgramMetrics} & Tracks program load statistics. \\
\hline
\code{reloading}: \code{bool} & Indicates if this is a reloading of an existing entry. \\
\hline
\end{tabular}

Once the ProgramCacheEntry is initialized, the program’s ELF bytecode is parsed and loaded into an Executable<InvokeContext<'static>>. This process involves calls Executable::load(), which takes in the ELF bytes and the ProgramRuntimeEnvironment. It calls:

\begin{enumerate}
    \item elf.rs::load\_with\_parser(): Parses the ELF bytecode to extract metadata and locate the entrypoint, which calls
    \item elf.rs::parse\_ro\_section(): Parses read-only sections of the ELF binary.
\end{enumerate}

Once parsing is complete, Executable::load() returns an Executable<InvokeContext<'static>> object.

If the system supports JIT compilation, the program is compiled to native machine code to optimize execution. JIT compilation occurs only if the underlying machine’s architecture is x86\_64 (Intel 64-bit processors) and not running Windows.

If these conditions are met, the program is compiled to native code via executable.jit\_compile(). This step significantly boosts performance by avoiding repeated interpretation of eBPF bytecode.

Preparing the Program Cache for a Transaction Batch

When transactions are processed, the Program Cache for a batch is prepared in svm::transaction\_processor.rs::TransactionBatchProcessor::load\_and\_execute\_sanitized\_transactions(). Here, the required programs are fetched and loaded ahead of batch execution to ensure efficient parallel execution.

Aside: Loading Built-in Programs at Bank Initialization

Some built-in programs (such as SystemProgram or VoteProgram) are not stored on-chain but are bundled directly with the validator.

When a new Bank is initialized (runtime::bank.rs::Bank::new\_from\_fields() or new\_with\_paths()), finish\_init() is called, which then calls ProgramCacheEntry::new\_builtin(). This loads builtin functions from the builtin function registry into the program cache so that they are immediately available.
